# Supplementary material for: DenRAM: Neuromorphic Dendritic Architecture with RRAM for Efficient Temporal Processing with Delays
Source: arXiv:2312.08960 source file (2023-12-14)

## a) Threshold Block

Schmitt Trigger

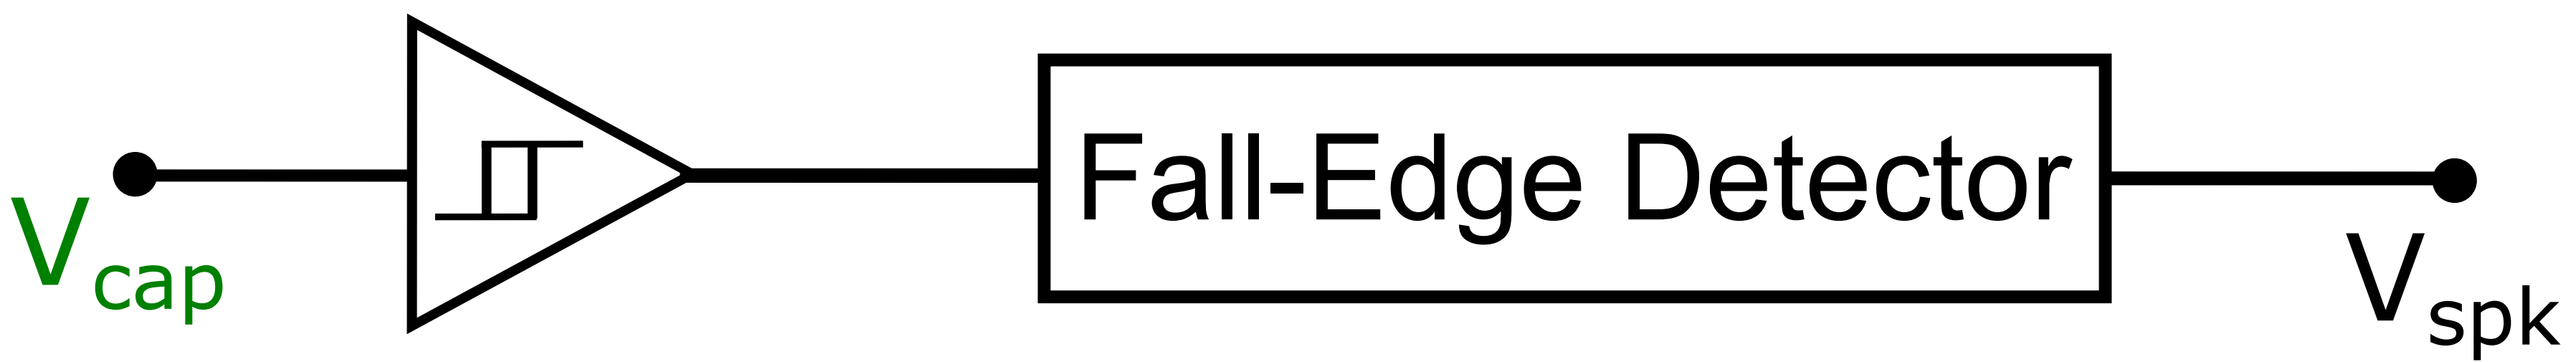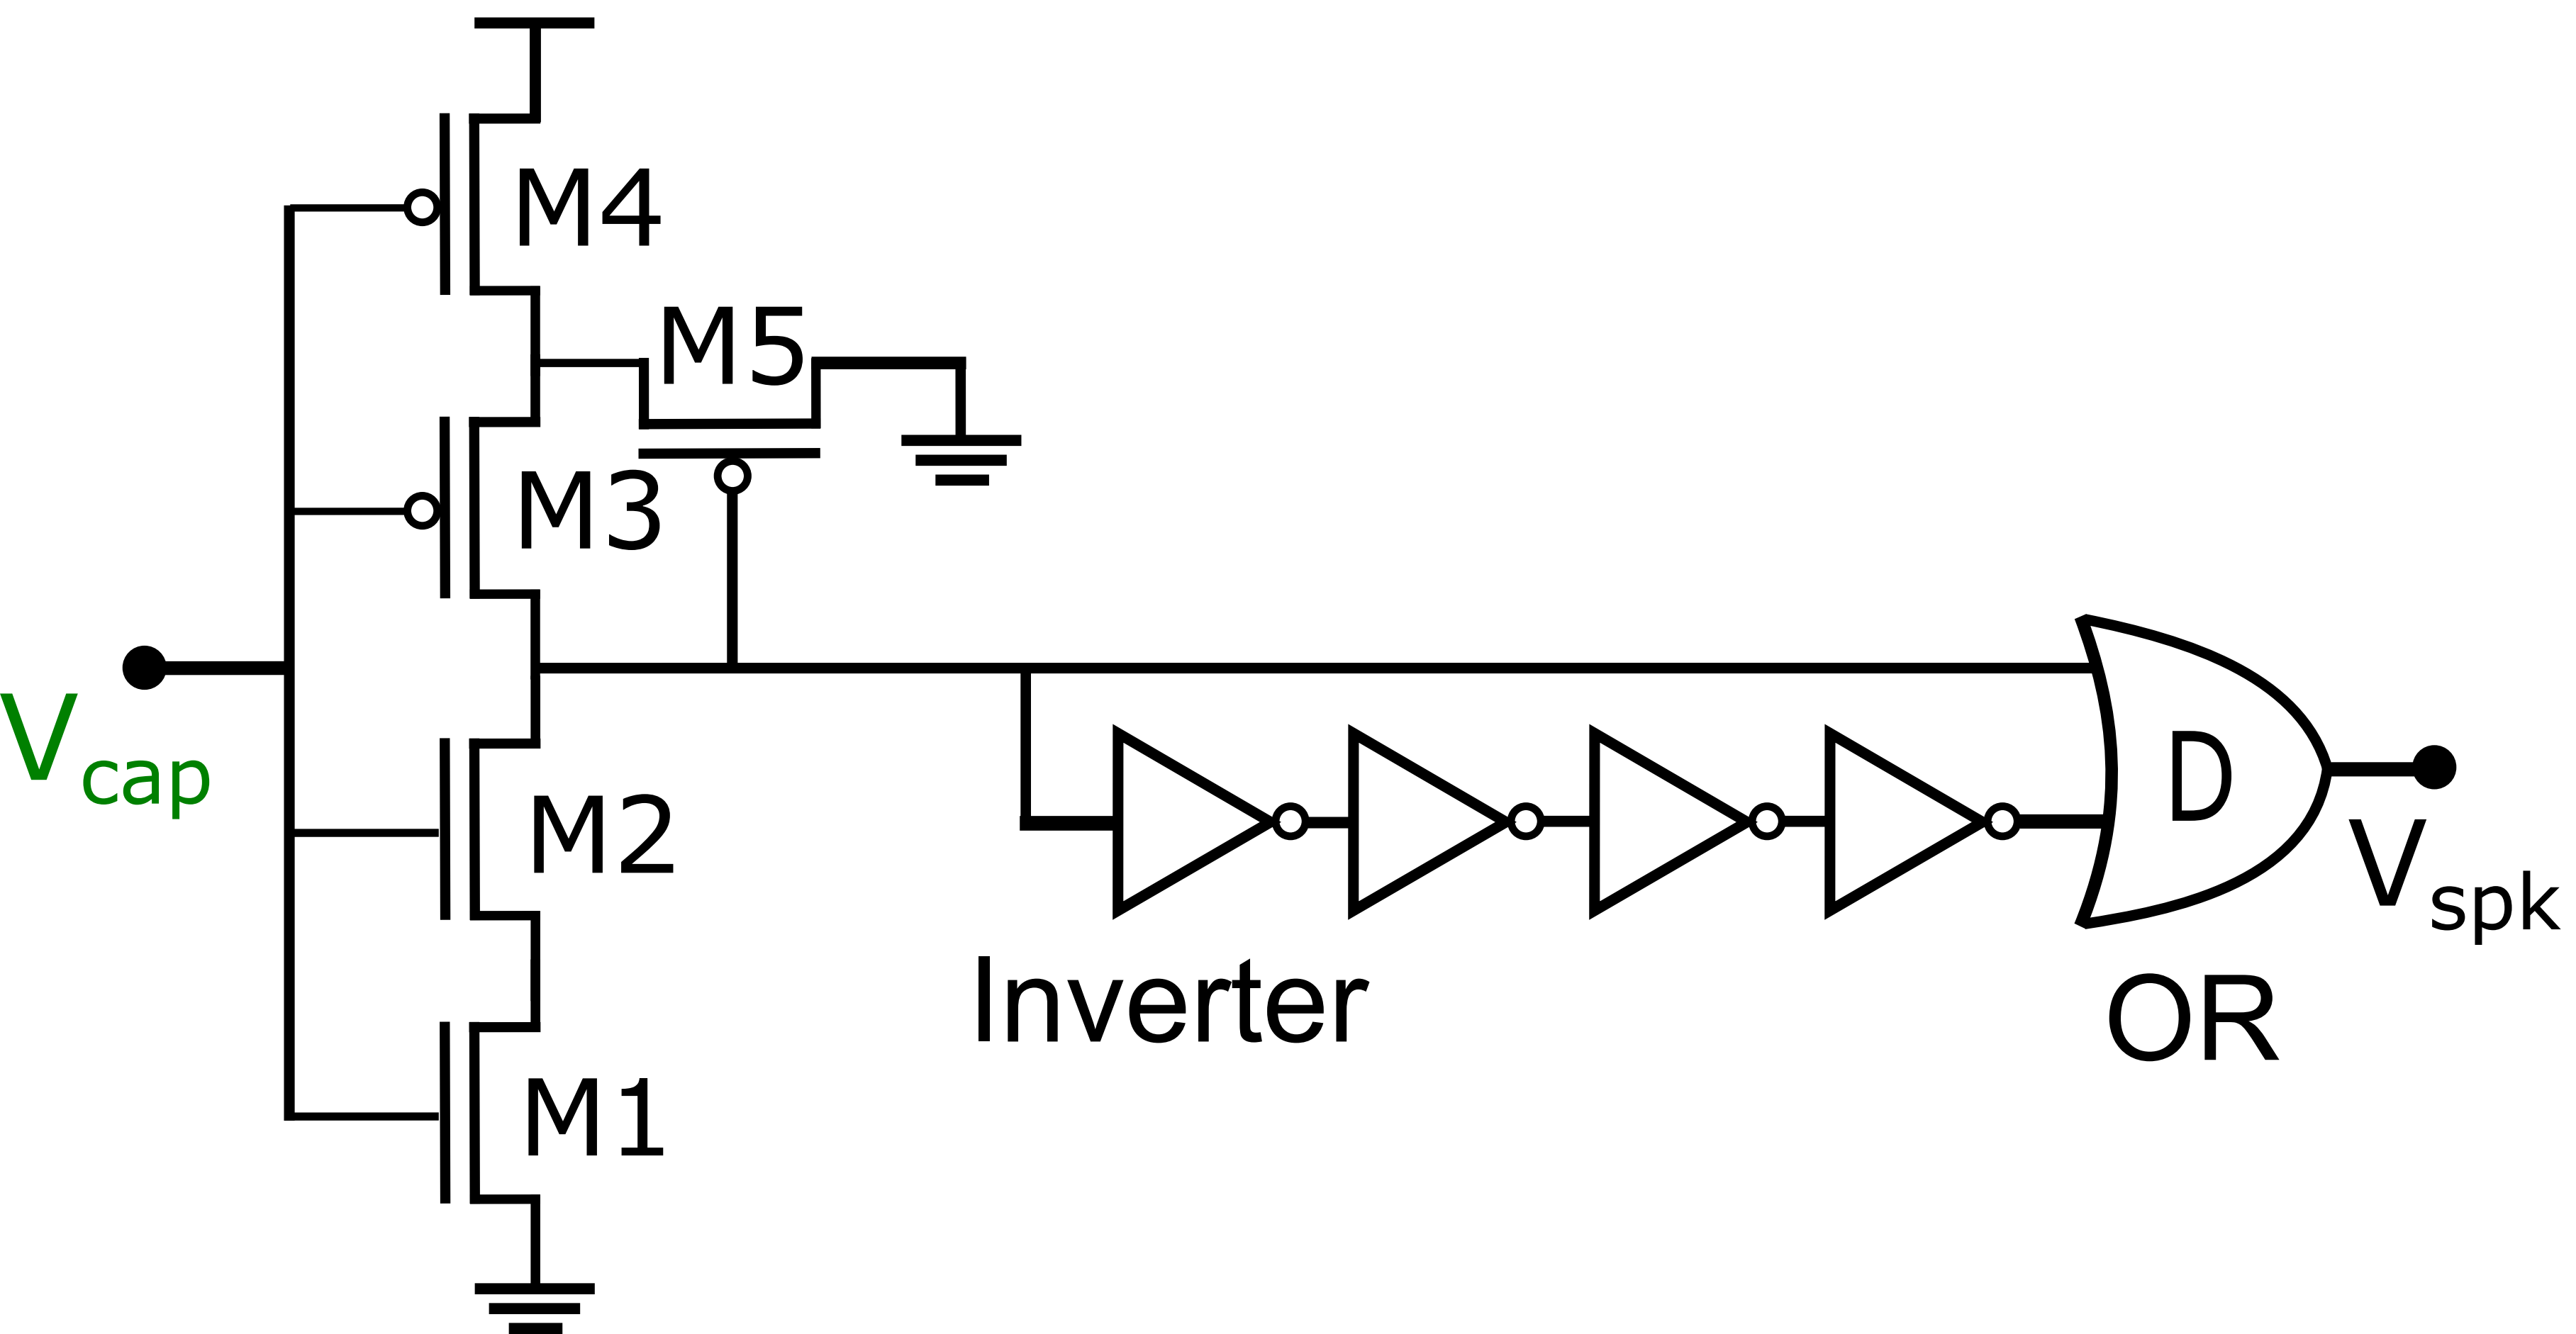

## b) LIF Neuron

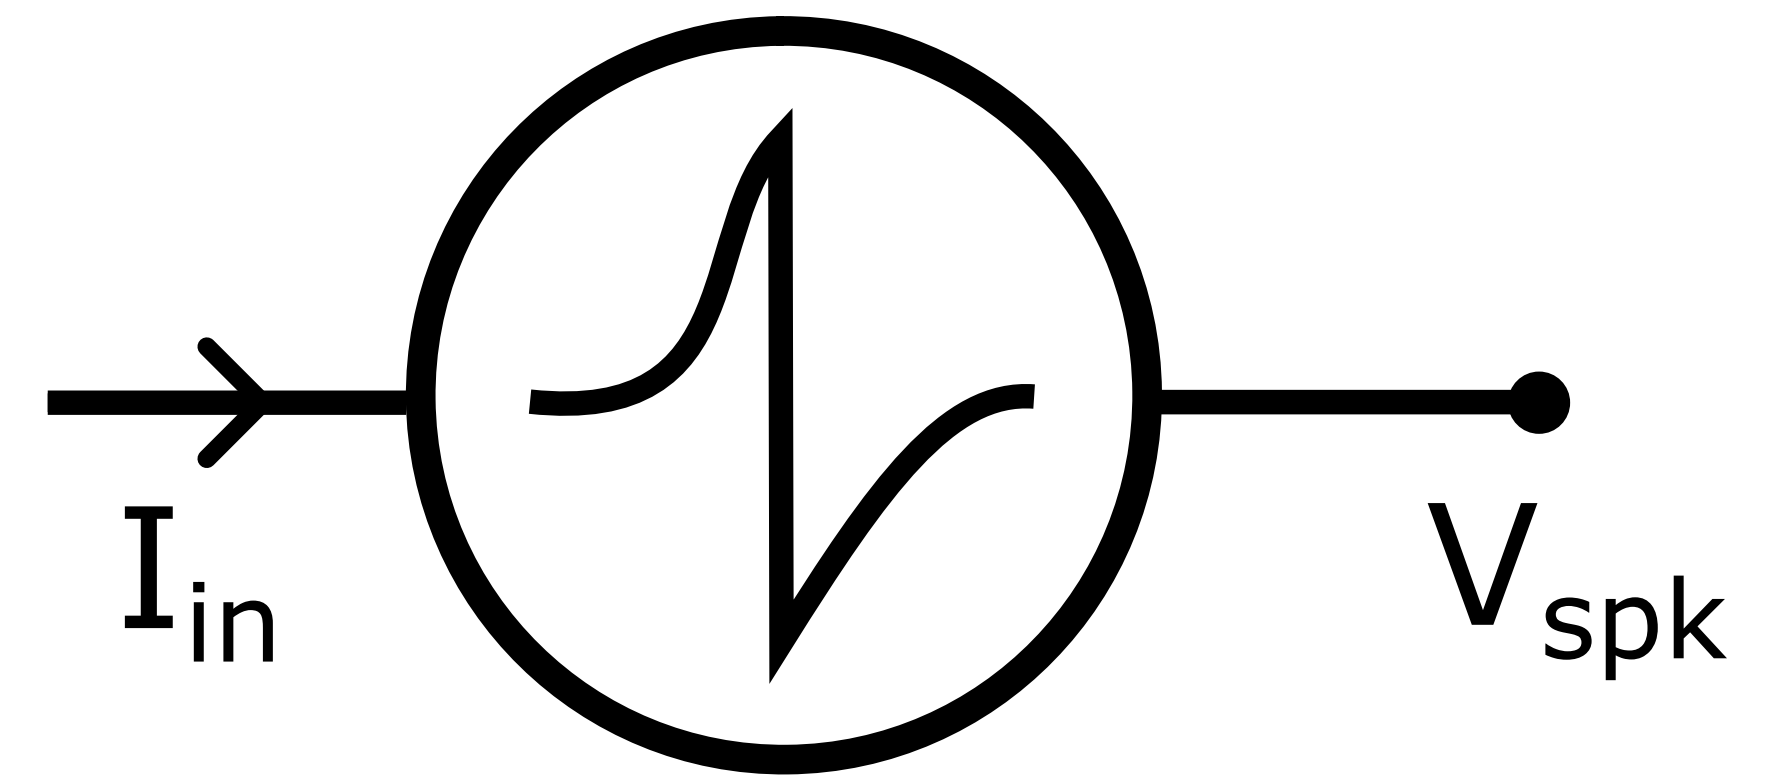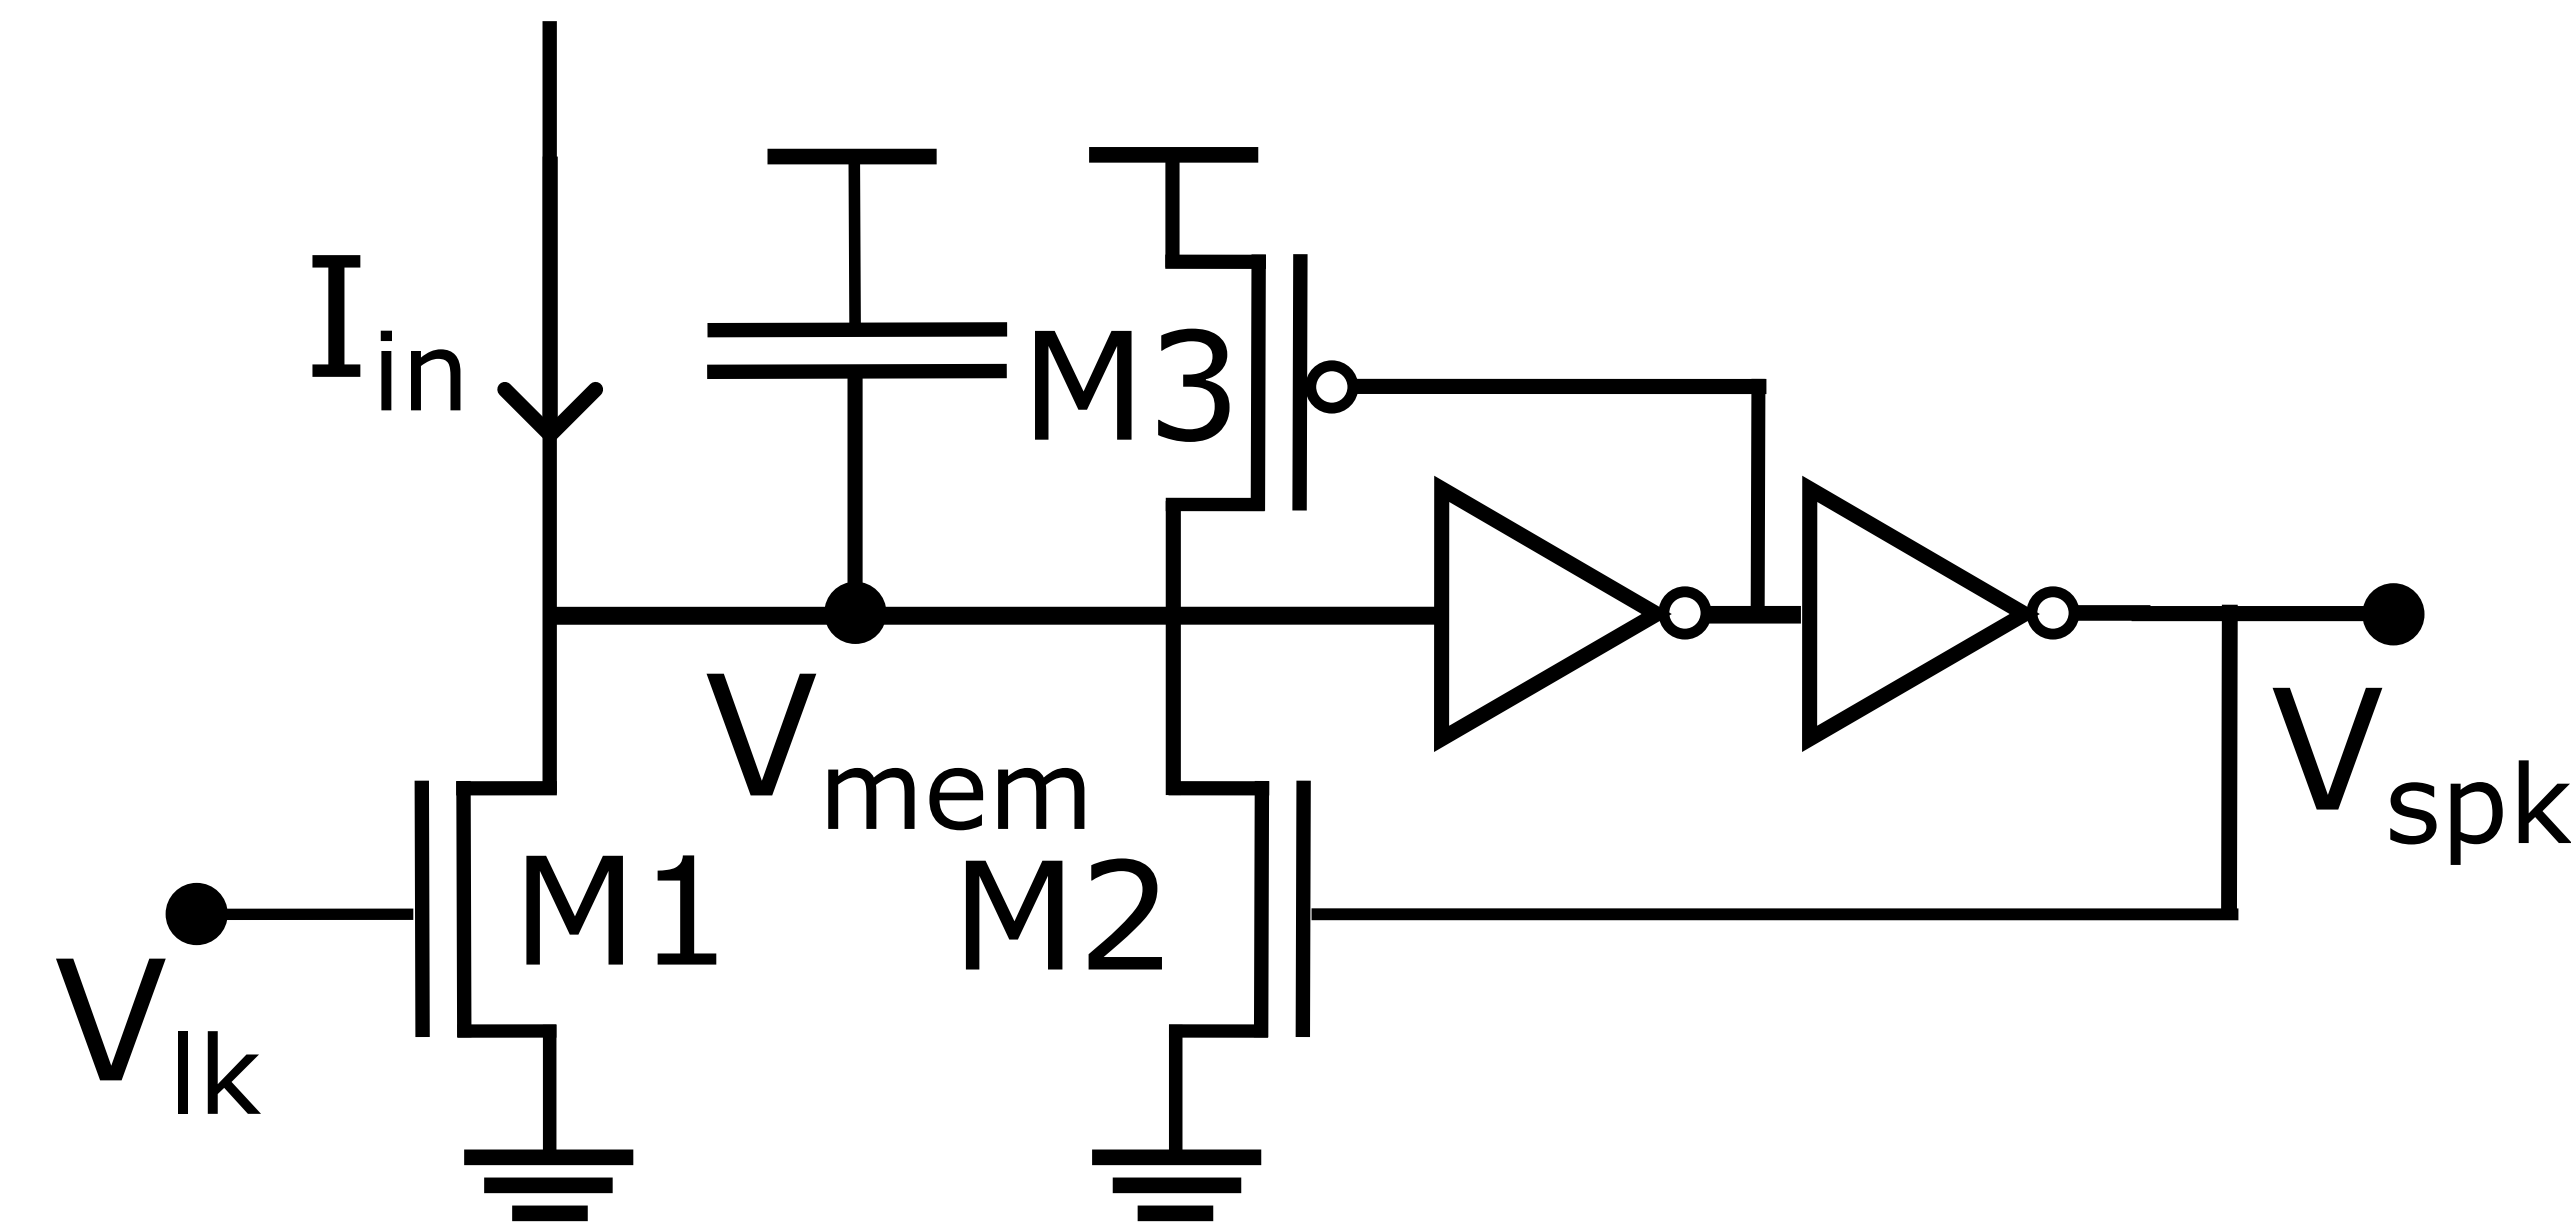

Supplement: Supplementary file 2 [file Figure_Suppl5_circuit.pdf]
